# Supplementary material for: Computing-specific pedagogies and theoretical models: common uses and relationships
Source: arXiv:2409.12245 source file (2024-08-22)
Supplement: Supplementary file 1 [file AppendixInstruments.tex]

\begin{table*}[hbpt]
\centering
\begin{tabular}{p{0.20\linewidth} p{0.44\linewidth} p{0.22\linewidth} r}

\multicolumn{4}{p{1.0\linewidth}}%
{\textbf{B} Instruments found in the study; ordered alphabetically by author name  within area of focus, and showing number of citations in Google Scholar as at 31 December 2022} \\

\toprule \textbf{Source paper} & \textbf{Theoretical construct}  &  \textbf{Methods} & \textbf{Citations} \\ \midrule

% \begin{center}
% \begin{longtable}{p{0.20\linewidth} p{0.44\linewidth} p{0.24\linewidth} r}
% %\caption{Instruments found in the study} \label{tab:instruments} \\
%   \label{tab:instruments}

% \toprule \textbf{Source paper} & \textbf{Instrument} & \textbf{Methods} & \textbf{Citations} \\ \midrule 
% \endfirsthead

% \multicolumn{4}{l}%
% {Instruments found in the study ... \textit{continued from previous page}} \\
% \toprule \textbf{Source paper} & \textbf{Instrument} & \textbf{Methods} & \textbf{Citations} \\  \midrule 
% \endhead

% \midrule \multicolumn{3}{r}{{\textit{continued on next page} ...}} \\
% \endfoot

% \bottomrule
% \endlastfoot

\multicolumn{3}{l}{\textbf{{Area of focus: assessment/self-assessment}}} \\
\citet{alaoutinen2012evaluating} & Taxonomy-based scale for self-evaluation of programming knowledge & used theory, empirical & 22 \\
\citet{basu2021principled} & Two instruments to assess 4th-6th grade students' CT skills & literature, factor analysis, empirical & 8\\
\citet{duran2019exploring} &  Instrument for self-evaluation of knowledge of programming concepts & adapted theory, exploratory \& confirmatory factor analysis, empirical & 12 \\
\citet{hogenboom2022computerized} & Computerized Adaptive Programming Concepts Test (CAPCT) to measure comprehension of basic sequences, loops, if statements, if-else statements, procedures, multiple agents, debugging, and generalization to a different programming syntax & empirical & 5 \\
\citet{kunkle2016impact} & Instrument to measure understanding of fundamental and object-oriented programming concepts & modified instrument, exploratory factor analysis, empirical  & 85 \\
\citet{parker2022pair} & New isomorphic versions of ACES assessment tool (Assessment of Computing for Elementary Students) & empirical & 1\\
\citet{porter2019bdsi} & Basic Data Structures Inventory (BDSI): validated concept inventory for assessing knowledge of basic data structures concepts & qualitative, empirical, CTT (classical test theory), IRT (item response theory) & 42 \\
    \citet{poulsen2021psychometric} & Cybersecurity concept inventory (validated in this paper) & delphi method, CTT, IRT & 2\\
\citet{ruiter2022coding} & Instrument for assessing young children's proficiency in the programming language ScratchJr. & used \& adapted theory, CTT, IRT & 20 \\

\multicolumn{3}{l}{\textbf{{Area of focus: teaching/pedagogical content knowledge}}} \\
\citet{ni2021understanding} & Instrument for assessing computer science teachers’ professional identity & used theory, exploratory \& confirmatory factor analysis & 4 \\
\citet{yadav2019computer} & Instrument to measure teachers computer science pedagogical content knowledge (Rasch model used) & literature, content analysis, empirical & 41\\
\citet{zhou2020high} & Instrument to measure high school teachers' self-efficacy to teach computer science & used theory, confirmatory factor analysis,  & 17\\

\end{tabular}
\end{table*}

%\end{longtable}
%\end{center}
%\footnote{CTT} Classical Test Theory
%\footnote{IRT} Item Response Theory
   
%\end{document}
