# Supplementary material for: Computing-specific pedagogies and theoretical models: common uses and relationships
Source: arXiv:2409.12245 source file (2024-08-22)
Supplement: Supplementary file 2 [file AppendixTCs.tex]

\begin{table*}[hbpt]
\centering
%\begin{longtable}{p{0.20\linewidth} p{0.44\linewidth} p{0.22\linewidth} r}
\begin{tabular}{p{0.20\linewidth} p{0.44\linewidth} p{0.22\linewidth} r}
%\caption{Instruments found in the study} \label{tab:instruments} \\
%\label{tab:instruments} 
\multicolumn{4}{p{1.0\linewidth}}%
{\textbf{A} Theoretical constructs, other than instruments, found in the study; ordered alphabetically by author name within area of focus, and showing number of citations in Google Scholar as at 31 December 2022} \\

\toprule \textbf{Source paper} & \textbf{Theoretical construct}  &  \textbf{Methods} & \textbf{Citations} \\ \midrule 
%\endfirsthead

% \multicolumn{4}{l}%
% {Theoretical constructs, other than instruments, found in the study ... \textit{continued from previous page}} \\
% \toprule \textbf{Source paper} & \textbf{Theoretical construct} & \textbf{Methods} & \textbf{Citations} \\  \midrule 
% \endhead

% \midrule \multicolumn{4}{r}{{\textit{continued on next page} ...}} \\
% \endfoot

% \bottomrule
% \endlastfoot

\multicolumn{3}{l}{\textbf{{Area of focus: assessment/self-assessment}}} \\
\citet{hundhausen2022assessing} & Regression model (extending Buffardi's model~\cite{buffardi2020assessing}) of the effect of a team member's GitHub contributions to the project grade & regression & 1 \\
% if we mentiond Buffardi here we need a citation - could leave out mention?
\citet{sheard2011exploring} & Classification scheme to investigate characteristics of introductory programming exam questions & argumentation, empirical &  48 \\
\citet{tahaei2018automated} & Logistic regression model for detecting plagiarism in programming assessments based on patterns of resubmission & literature, argumentation, regression, empirical &  22 \\

\multicolumn{3}{l}{\textbf{{Area of focus: content/curriculum/learning goals}}} \\

\citet{cutts2012abstraction} & Abstraction transition (AT) taxonomy to classify the knowledge and practices required to apprentice students into the programming community & argumentation, empirical & 46 \\
\citet{goldman2010setting} & Lists of expert-identified central concepts for programming fundamentals, discrete math, and logic design & delphi method & 99 \\
\citet{sharmin2021creativity} & Components of creativity-enhancing activities & literature, argumentation & 5 \\
\citet{thayer2021theory} & A theory of components of API knowledge & argumentation, regression & 17 \\
\citet{werner2020computational} & GCS 2.0 (game computational sophistication): measure of the relationship between different types of building blocks of computer games and game computational sophistication; new version of the GCS~\cite{werner2014children} & extended model,  argumentation, empirical & 8 \\

\multicolumn{3}{l}{\textbf{{Area of focus: teaching/pedagogical content knowledge}}} \\
\citet{ahmad2020impact} & A gamification framework from literature & extended theory, argumentation, empirical & 42 \\
\citet{carbone2007CSandIT} & Two outcome spaces: IT academics conceptions of successful teaching (3 categories) and  IT academics conceptions of unsuccessful teaching (5 categories) & phenomenography & 44\\
\citet{clarke2021combining} & Model for maximizing the use of learning and engagement strategies & literature, argumentation, empirical & 1\\
\citet{duran2021rules} & A framework for identifying, organizing, and communicating learning objectives that involve program semantics & literature, argumentation & 6 \\
\citet{margulieux2021wrong} & Multiple conceptions theory - a framework which allows analysis of various generic pedagogies and explanation of their differences & used theory, literature, argumentation & 9 \\
\citet{rich2022learning} & Learning trajectory for variables & extended model, literature, argumentation & 7\\
\citet{sentance2021teachers} & A model to frame understanding of how programming teachers use classroom talk to support the learning of programming &  phenomenography, thematic analysis & 4 \\
\citet{sharma2022usually} & A model of systemic misalignments in implementing undergraduate research experiences & grounded theory & 0\\
\citet{steghofer2018involving} & Two models: A model for analysing involvement of external stakeholders in university courses and a model to design actions & action research & 4 \\
\citet{tutty2008teaching} & Five categories of teaching experience and practice & phenomenography & 25 \\
\citet{xie2019theory} & A holistic theory for teaching programming by splitting it into several skills & used theory, literature, argumentation & 87\\

\end{tabular}
\end{table*}

%\end{longtable}
%\end{center}
